# Supplementary material for: NVBleed: Covert and Side-Channel Attacks on NVIDIA Multi-GPU Interconnect
Source: arXiv:2503.17847 source file (2025-03-22)
Supplement: Supplementary file 1 [file appendix.tex]

\section{Appendix}
\label{sec:appendix}

We provide definitions for the OpenMM benchmarks, NVLink-related performance counters, and statistical features utilized in \textit{NVBleed} in Tables~\ref{tb:benchmark_description}, Table~\ref{tb:counter_definition}, Table~\ref{tb:features_definition}, respectively. Additionally, Table~\ref{tb:dnn_models} presents the deep learning models evaluated under \textit{NVBleed}, while Table~\ref{tb:hp-classifier} showcases the hyper-parameter settings for the classifiers used in \textit{NVBleed}.

\begin{table*}[]
\centering
\small
\caption{Descriptions of OpenMM benchmarks~\cite{openmmbenchmark}.}
\label{tb:benchmark_description}
\begin{tabular}{|L{2.5cm}|L{15cm}|}
\hline
\textbf{OpenMM}                             & \textbf{Description}                                                                                                                                \\ \hline \hline
 rf & The rf benchmark focuses on dihydrofolate reductase (DHFR) models, with long-range interactions truncated at 1 nm using the Reaction Field (RF) method.
\\  \hline 
  pme &  The pme benchmark concentrates on DHFR models, with long-range interactions calculated using the Particle Mesh Ewald (PME) method.
\\  \hline 
   apoa1-rf & The apoa1-rf benchmark focuses on Apolipoprotein A1 (ApoA1), with long-range interactions truncated at 1 nm using the RF method.
   \\ \hline
    apoa1-pme & The apoa1-pme benchmark concentrates on ApoA1, with long-range interactions calculated using the PME method.
    \\ \hline
  apoa1-ljpme & The apoa1-ljpme benchmark concentrates on ApoA1. Particle Mesh Ewald was used for both Coulomb and Lennard-Jones interactions.
  \\ \hline
   amoeba-pme &  The amoeba-pme benchmark is built on the DHFR models with the AMOEBA polarizable force field. The PME method was used to model long range interactions.
   \\ \hline
    amber20-dhfr & The amoeba-dhfr benchmark is built on the DHFR models taken from the Joint Amber/Charmm benchmark~\cite{salomon2013overview}.
    \\ \hline
  amber20-cellulose & The amber20-cellulose is built on the cellulose model taken from the Joint Amber/Charmm benchmark.
  \\ \hline

\end{tabular}

\end{table*}

\begin{table*}[]
\centering
% \small
\caption{Definitions of NVLink-related performance counters.}

\begin{tabular}{|l|l|}
\hline
\textbf{Counters}                             & \textbf{Definition}                                                                                                                                \\ \hline \hline
% nvlink\_overhead\_data\_received/transmitted  & Ratio of overhead data to the total data, received/transmitted through NVLink.                                                                     \\ \hline
nvlink\_receive/transmit\_throughput          & Number of bytes received per second through NVLinks.                                                                                               \\ \hline
nvlink\_user\_data\_received/transmitted      & User data bytes received through NVLinks, doesn't include headers.                                                                                 \\ \hline
nvlink\_user\_write\_data\_transmitted        & User write data bytes transmitted through NVLinks.                                                                                                 \\ \hline
nvlink\_user\_response\_data\_received        & Total user response data bytes received through NVLink. \\ \hline
nvlink\_total\_data\_received/transmitted     & Total data bytes received/transmitted through NVLinks including headers.                                                                           \\ \hline
nvlink\_total\_response\_data\_received       & Total response data bytes received through NVLink.      \\ \hline
nvlink\_total\_write\_data\_transmitted       & Total write data bytes transmitted through NVLinks.                                                                                                \\ \hline
nvlink\_total/user\_nratom\_data\_transmitted & Total/User non-reduction atomic data bytes transmitted through NVLinks.                                                                            \\ \hline
nvlink\_total/user\_ratom\_data\_transmitted  & Total/User reduction atomic data bytes transmitted through NVLinks.                                                                                \\ \hline
\end{tabular}
\label{tb:counter_definition}
\end{table*}

\begin{table*}[]
\small
\centering
\caption{Hyper-parameter settings for classifiers}

\begin{tabular}{|L{2cm}|L{12cm}|}
\hline
\textbf{Classifiers} & \textbf{Settings}                                                                     \\ \hline \hline
KNN                  & $n\_neighbors = 5, leaf\_size = 30, p = 2, weights = uniform, metric= euclidean $ 
\\ \hline
XGBoost              & $n\_estimators = 100, booster = gbtree, learning\_rate=0.1, max\_depth=6, subsample=0.8    $ 
\\ \hline
LightGBM             & $boosting\_type = gbdt,num\_leaves = 31,max\_depth = -1,n\_estimators = 100, learning\_rate=0.1. subsample= 1.0 $ 
\\ \hline

\end{tabular}
\label{tb:hp-classifier}
\end{table*}

\begin{table*}[]
\small
\caption{Deep learning models evaluated under \textit{NVBleed}. \tabletitle{(Conv=\texttt{Convectional layer} and the subscripts of C stand for the size of the filter, number of filters, stride, and padding. FC=\texttt{Fully-connected layer} and the number of neurons in F are shown in subscript. P=\texttt{Pooling}, and its subscripts represent filter size and stride. LSTM=\texttt{LSTM layer}, and its subscripts represent hidden size.)} }
\centering
\begin{tabular}{|l|l|}
\hline

\textbf{Models} & \textbf{Description}                                                                     \\ \hline \hline
MLP                  &    $F_{512}-F_{256}-F_{10}$   
\\ \hline
CNN\_1              &  $C_{5,16,1,2}-P_{2,2}-F_{10}$
\\ \hline
CNN\_2              &  $C_{3,32,1,1}-P_{2,2}-C_{3,64,1,1}-P_{2,2}-C_{3,128,1,1}-P_{2,2}-F_{256}-F_{10}$
\\ \hline
Regression             & $F_{512}-F_{128}-F_{1}$   
\\ \hline
LSTM             &  $LSTM_{128}-F_{10}$ 
\\ \hline
AlexNet             & A famous CNN model (11 layers) in computer vision.
\\ \hline
VGG16             & A famous CNN model (16 layers) in computer vision.
\\ \hline
GoogLeNet             & A famous CNN model (22 layers) in computer vision.
\\ \hline
ResNet-18             &  A famous CNN model (18 layers) in computer vision.
\\ \hline
ResNet-50             & A famous CNN model (50 layers) in computer vision.
\\ \hline

\end{tabular}
% \vspace{10pt}

\label{tb:dnn_models}
\end{table*}
